# Supplementary material for: Bounding, Concentrating, and Truncating: Unifying Privacy Loss Composition for Data Analytics
Source: arXiv:2004.07223 source file (2020-11-17)
Supplement: Supplementary file 1 [file appendix.tex]

%!TEX root = main.tex

\section{Appendix \label{sec:appendix}} % (fold)
